# Supplementary material for: Microsimulation Model Calibration using Incremental Mixture Approximate Bayesian Computation
Source: arXiv:1804.02090 source file (2018-08-13)
Supplement: Supplementary file 1 [file appendix_additionalcalibrationresults.pdf]

# Supplementary Material for Microsimulation Model Calibration using Incremental Mixture Approximate Bayesian Computation

August 4, 2018

## 1 Additional CRC-SPIN 2.0 Calibration Results

Studies that were used for calibration purposes often included additional information not included as calibration targets. We compared model predictions of these results to gain additional insight into the performance of the calibrated model (Table 1). In general, these comparisons indicate that the calibrated model was able to recover key characteristics of target data.

- Although the model predicted higher adenoma prevalence than observed in the Corley et al. (2013) study, this was anticipated because this study was carried out in an insured population after the dissemination of CRC screening. While CRC screening remained low during this period (approximately 30%), it is plausible that some participants in this study had previously undergone colonoscopy. Two studies conducted during earlier time periods also provided information about adenoma prevalence (Pickhardt et al., 2003; Lieberman et al., 2000). The model predicted a similar number of adenomas per person in the Pickhardt et al. (2003) study, and similar adenoma prevalence as that observed by Lieberman et al. (2000).

- Based on location information provided in the Corley et al. (2013) study, we find that the model generally recovered the distribution of adenomas in the distal and proximal locations. The model predicts a somewhat higher prevalence of agents with both distal and proximal adenomas, especially in men. When we standardize the distribution of overall prevalence, we find that among women the model predicts that 19.8% of women with at least one adenoma have adenomas in both proximal and distal locations (versus 20.3% observed). Among men the model predicts that 42.0% with at least one adenoma have adenomas in both proximal and distal locations (versus 30.6% observed). It is difficult to determine how much this may be driven by screening, particularly since the health care system where this study was performed had an active program of screening via flexible simoidocopy. However, this may have implications for the model-predicted effectiveness of flexible sigmoidoscopy.

- The model may not replicate the continuous size distribution of simulated adenomas. For the Pickhardt et al. (2003) study, the model predicted too many small ($< 5$mm) adenomas

Table 1: Additional observed and predicted results, not used for calibration

| Target | Observed Mean | Posterior Predicted Mean | Posterior Predicted 95% CI |
|---|---|---|---|
| Corley et al. (2013) | | | |
| Prevalence, Only Distal Adenomas, Women | 8.9 | 11.0 | (9.7, 12.5) |
| Prevalence, Only Proximal Adenomas, Women | 8.3 | 10.9 | (7.8, 14.4) |
| Prevalence, Distal & Proximal Adenomas, Women | 3.1 | 5.4 | (3.2, 8.0) |
| Prevalence, Only Distal Adenomas, Men | 12.6 | 11.3 | (9.7, 13.2) |
| Prevalence, Only Proximal Adenomas, Men | 11.9 | 8.7 | (7.6, 9.9) |
| Prevalence, Distal & Proximal Adenomas, Men | 6.1 | 14.5 | (12.4,16.8) |
| Pickhardt et al. (2003)* | | | |
| Percent of Detected Adenomas $\leq$ 5mm | 62.0 | 75.1 | (73.2, 76.9) |
| Percent of Detected Adenomas $6-9$mm | 28.7 | 12.7 | (11.7, 14.1) |
| Average Number of Detected Adenomas Per Person | 0.45 | 0.49 | (0.35, 0.71) |
| Number of Preclinical Cancers per 1,000 People | 1.6 | 2.1 | (1.5, 3.0) |
| Lieberman et al. (2008)* | | | |
| Preclinical CRCs per 1,000 Lesions $<$ 6mm | 0.55 | 0.10 | (0.01, 0.23) |
| Adenoma Prevalence | 26.0 | 27.2 | (24.6,30.8) |
| Percent of Adenomas $\geq$ 10mm that are 10-14mm | 71.4 | 55.7 | (51.5,60.2) |
| Percent of Adenomas $\geq$ 10mm that are 15-20mm | 16.6 | 25.3 | (24.5,26.2) |
| Percent of Adenomas $\geq$ 10mm that are 20-25mm | 8.7 | 11.3 | (9.7,12.62) |
| Percent of Adenomas $\geq$ 10mm that are $>$ 25mm | 3.2 | 7.7 | (5.2,10.7) |
| Church (2004) | | | |
| Preclinical CRCs per 1,000 Lesions $<$ 6mm | 0.97 | 0.12 | (0.03,0.27) |

*Size was reported categorically as $\leq$ 5mm, 6 to 9mm, and $\geq$ 10mm. We operationalized these categories as: $[1, 5.5)$ mm, $[5.5, 9.5)$ mm and $\geq 9.5$ mm

and too few adenomas that are 6 to 9mm. From the Lieberman et al. (2000) study, the model predicted too few adenomas 10-14mm, and too many adenomas $>$ 15mm. However, it is difficult to determine the source and importance of this possible misalgnment. First, the model predicted continuous size, but studies reported discrete size categories such that adenomas from 5 to 6mm and from 9 to 10mm were not explicitly assigned to a category. Second, adenoma size is measured with error that is not accounted for by the model (**??**).

- There was also some indication that the model may predict too few cancers in adenomas $<$ 6mm. However, it is difficult to determine the impact of this given potential errors in observed adenoma sizes. In addition, we found that the model may predict too many cancers in adenomas 6-9mm (as reported in the main paper).

## 1.1 Estimated Posterior Distributions

Posterior distributions update prior distributions specified for model parameters using observed data. The figures in this section show both prior and posterior distribution estimates to demonstrate this updating.

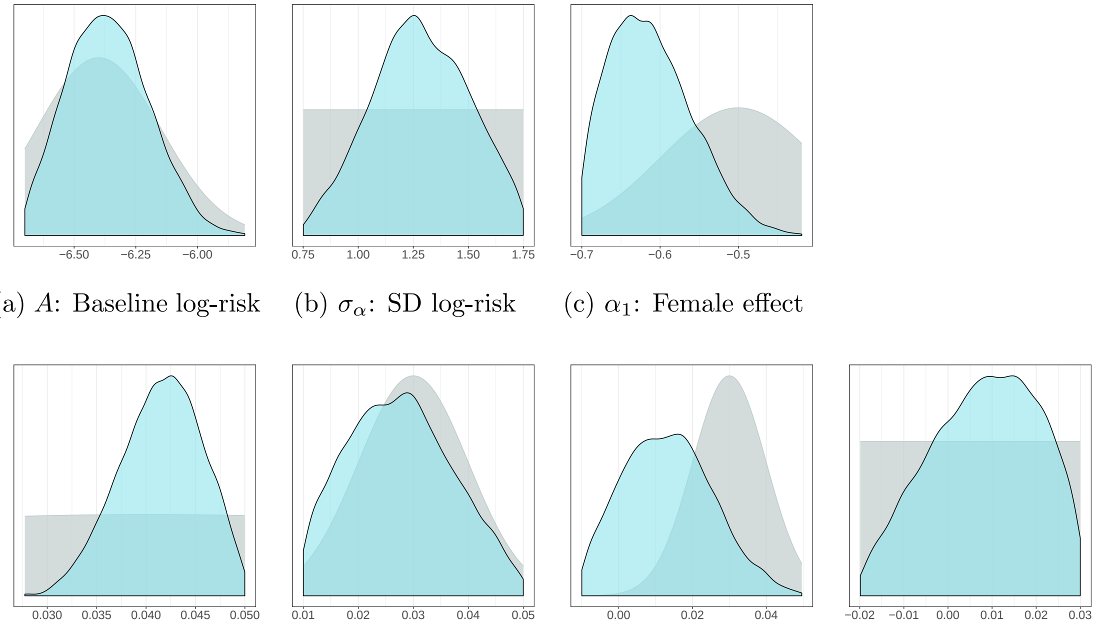


(a) $A$: Baseline log-risk (b) $\sigma_\alpha$: SD log-risk (c) $\alpha_1$: Female effect

(d) $\alpha_{20}$: Age [20,50) (e) $\alpha_{50}$: Age [50,60) (f) $\alpha_{60}$: Age [60,70) (g) $\alpha_{70}$: Age $\geq 70$

Figure 1: Posterior and prior distributions of adenoma risk parameters.

Posterior estimates demonstrate prior to posterior learning for most parameters. We had considerable prior information about baseline adenoma risk, and so it is not suprizing to see similarity between prior and posterior distributions for this parameter (Figure 3a). There is some suggestion that interaction terms in the adenoma transition model ($\gamma_5$, $\gamma_6$, and $\gamma_7$) may be dropped from the model, though this would require recalibration. There was also some indication that the colon scale parameter, $\beta_{2C}$ was constrained by the upper limit of its prior range, and that MST parameters were constrained by the lower limit of their prior ranges.

## 1.2 Posterior Correlations

Table 2 shows correlations between the 21 parameters in the CRC-spin model, rounded to two decimal places. Correlations that exceed 0.5 in absolute value are bolded (excluding those on the diagonal which are all by definition equal to 1). The estimated correlations are useful for understanding the interplay between the many parameters of the various model components. For instance, the shape and scale parameters of the Fréchet distribution for adenoma growth in the rectum ($\beta_{1R}$ and $\beta_{2R}$) are negatively correlated. This makes sense, because if one of these parameters shifts up or down, the other must also change to allow for an adequate amount of skewness and a right-tail that accommodates slow-growing adenomas. However, there are also less obvious correlations that present themselves, like those between the parameters of the adenoma risk model and the growth model (e.g., $\gamma_2$ and $\beta_{2R}$, and $\gamma_2$ and $\beta_{1R}$), which suggest that adenoma risk impacts features of adenoma growth.

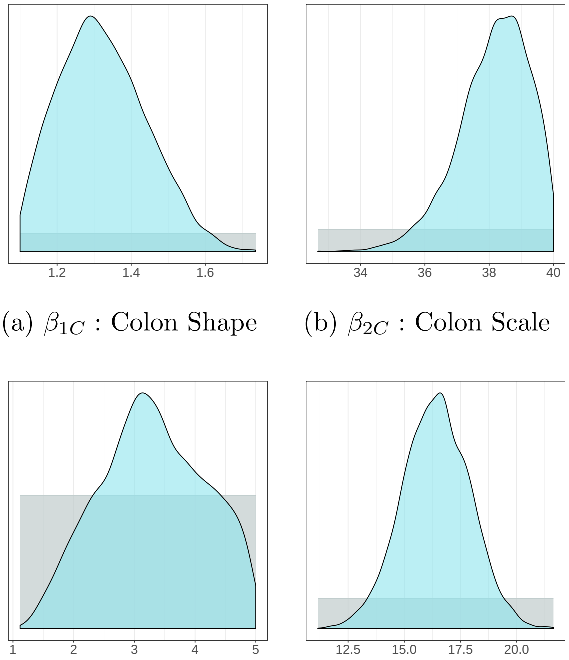


(a) $\beta_{1C}$ : Colon Shape (b) $\beta_{2C}$ : Colon Scale

(c) $\beta_{1R}$ : Rectum Shape (d) $\beta_{2R}$ : Rectum Scale

Figure 2: Posterior and prior distributions of adenoma growth parameters.

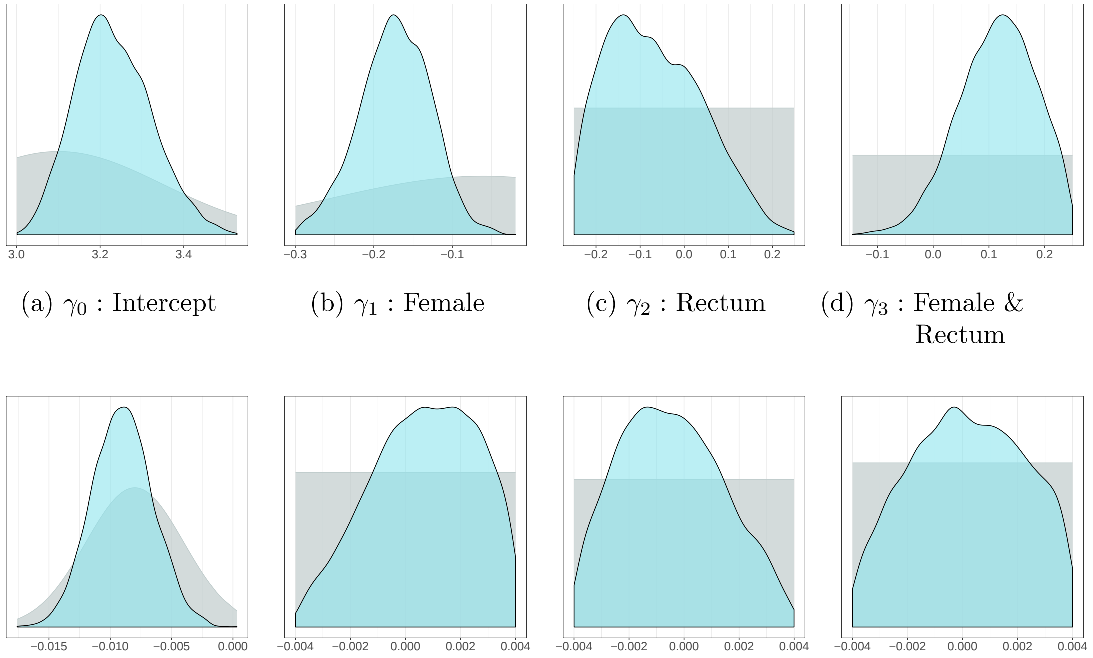


(a) $\gamma_0$ : Intercept (b) $\gamma_1$ : Female (c) $\gamma_2$ : Rectum (d) $\gamma_3$ : Female & Rectum

(e) $\gamma_4$ : Initiation Age (f) $\gamma_5$ : Initiation Age $\times$ Female (g) $\gamma_6$ : Initiation Age $\times$ Rectum (h) $\gamma_7$ : Initiation Age $\times$ Female & Rectum

Figure 3: Posterior and prior distributions of adenoma transitions parameters. Top row shows intercept terms and main effects. Bottom row shows age at initiation and interactions with age.

Table 2: Correlations between parameters of the CRC-SPIN model, estimated through sample correlations based on posterior draws. Correlations that exceed 0.5 in absolute value are bolded.

| | $A$ | $\alpha_1$ | $\sigma_\alpha$ | $\alpha_{20}$ | $\alpha_{50}$ | $\alpha_{60}$ | $\alpha_{70}$ | $\beta_{1C}$ | $\beta_{2C}$ | $\beta_{1R}$ | $\beta_{2R}$ | $\gamma_0$ | $\gamma_1$ | $\gamma_2$ | $\gamma_3$ | $\gamma_4$ | $\gamma_5$ | $\gamma_6$ | $\gamma_7$ | $\tau_C$ | $\tau_R$ |
|---|---|---|---|---|---|---|---|---|---|---|---|---|---|---|---|---|---|---|---|---|---|
| $A$ | 1.00 | 0.09 | -0.45 | **-0.61** | -0.09 | -0.06 | 0.20 | 0.18 | 0.14 | 0.04 | -0.13 | -0.39 | 0.13 | 0.24 | -0.10 | -0.14 | 0.08 | -0.03 | -0.09 | 0.05 | -0.03 |
| $\alpha_1$ | 0.09 | 1.00 | -0.08 | -0.25 | 0.06 | 0.02 | 0.08 | 0.09 | 0.06 | 0.27 | -0.22 | -0.23 | 0.42 | 0.11 | 0.16 | 0.13 | -0.14 | -0.08 | -0.07 | 0.02 | 0.18 |
| $\sigma_\alpha$ | -0.45 | -0.08 | 1.00 | -0.14 | 0.19 | 0.15 | -0.20 | -0.08 | 0.12 | -0.25 | 0.40 | **0.57** | 0.04 | -0.27 | 0.17 | -0.06 | -0.12 | -0.09 | 0.14 | 0.28 | 0.15 |
| $\alpha_{20}$ | **-0.61** | -0.25 | -0.14 | 1.00 | -0.33 | -0.14 | -0.16 | -0.17 | -0.21 | 0.04 | 0.00 | 0.42 | -0.22 | -0.14 | -0.07 | 0.39 | -0.03 | 0.01 | 0.15 | -0.18 | -0.11 |
| $\alpha_{50}$ | -0.09 | 0.06 | 0.19 | -0.33 | 1.00 | 0.08 | -0.04 | -0.08 | 0.13 | 0.07 | 0.01 | -0.15 | 0.09 | 0.02 | 0.07 | -0.17 | 0.12 | 0.32 | -0.07 | 0.14 | 0.03 |
| $\alpha_{60}$ | -0.06 | 0.02 | 0.15 | -0.14 | 0.08 | 1.00 | -0.15 | -0.15 | 0.07 | -0.30 | 0.15 | 0.03 | 0.06 | -0.22 | 0.01 | -0.15 | -0.15 | -0.05 | 0.10 | -0.03 | 0.10 |
| $\alpha_{70}$ | 0.20 | 0.08 | -0.20 | -0.16 | -0.04 | -0.15 | 1.00 | 0.33 | -0.15 | 0.29 | -0.29 | -0.31 | 0.12 | 0.34 | -0.10 | 0.06 | 0.29 | -0.12 | -0.24 | -0.11 | 0.06 |
| $\beta_{1C}$ | 0.18 | 0.09 | -0.08 | -0.17 | -0.08 | -0.15 | 0.33 | 1.00 | -0.48 | 0.30 | -0.17 | -0.39 | 0.26 | 0.43 | -0.05 | 0.37 | 0.31 | -0.11 | -0.12 | -0.17 | 0.23 |
| $\beta_{2C}$ | 0.14 | 0.06 | 0.12 | -0.21 | 0.13 | 0.07 | -0.15 | -0.48 | 1.00 | 0.01 | -0.02 | -0.06 | -0.10 | 0.11 | 0.07 | -0.27 | -0.22 | 0.11 | -0.01 | 0.06 | -0.09 |
| $\beta_{1R}$ | 0.04 | 0.27 | -0.25 | 0.04 | 0.07 | -0.30 | 0.29 | 0.30 | 0.01 | 1.00 | **-0.55** | -0.30 | 0.16 | **0.58** | 0.00 | 0.29 | 0.13 | 0.21 | -0.13 | -0.24 | -0.01 |
| $\beta_{2R}$ | -0.13 | -0.22 | 0.40 | 0.00 | 0.01 | 0.15 | -0.29 | -0.17 | -0.02 | **-0.55** | 1.00 | 0.36 | -0.08 | **-0.75** | -0.11 | -0.08 | -0.24 | -0.01 | 0.22 | 0.16 | -0.15 |
| $\gamma_0$ | -0.39 | -0.23 | **0.57** | 0.42 | -0.15 | 0.03 | -0.31 | -0.39 | -0.06 | -0.30 | 0.36 | 1.00 | -0.29 | -0.47 | 0.04 | 0.30 | -0.27 | -0.14 | 0.31 | 0.21 | -0.06 |
| $\gamma_1$ | 0.13 | 0.42 | 0.04 | -0.22 | 0.09 | 0.06 | 0.12 | 0.26 | -0.10 | 0.16 | -0.08 | -0.29 | 1.00 | 0.10 | 0.02 | -0.03 | 0.38 | -0.03 | -0.09 | -0.00 | 0.26 |
| $\gamma_2$ | 0.24 | 0.11 | -0.27 | -0.14 | 0.02 | -0.22 | 0.34 | 0.43 | 0.11 | **0.58** | **-0.75** | -0.47 | 0.10 | 1.00 | -0.18 | 0.12 | 0.26 | 0.19 | -0.30 | -0.10 | 0.01 |
| $\gamma_3$ | -0.10 | 0.16 | 0.17 | -0.07 | 0.07 | 0.01 | -0.10 | -0.05 | 0.07 | 0.00 | -0.11 | 0.04 | 0.02 | -0.18 | 1.00 | -0.07 | -0.01 | -0.16 | 0.23 | -0.00 | 0.08 |
| $\gamma_4$ | -0.14 | 0.13 | -0.06 | 0.39 | -0.17 | -0.15 | 0.06 | 0.37 | -0.27 | 0.29 | -0.08 | 0.30 | -0.03 | 0.12 | -0.07 | 1.00 | -0.18 | -0.16 | 0.15 | -0.01 | 0.04 |
| $\gamma_5$ | 0.08 | -0.14 | -0.12 | -0.03 | 0.12 | -0.15 | 0.29 | 0.31 | -0.22 | 0.13 | -0.24 | -0.27 | 0.38 | 0.26 | -0.01 | -0.18 | 1.00 | 0.03 | -0.15 | -0.06 | 0.19 |
| $\gamma_6$ | -0.03 | -0.08 | -0.09 | 0.01 | 0.32 | -0.05 | -0.12 | -0.11 | 0.11 | 0.21 | -0.01 | -0.14 | -0.03 | 0.19 | -0.16 | -0.16 | 0.03 | 1.00 | -0.14 | -0.13 | -0.21 |
| $\gamma_7$ | -0.09 | -0.07 | 0.14 | 0.15 | -0.07 | 0.10 | -0.24 | -0.12 | -0.01 | -0.13 | 0.22 | 0.31 | -0.09 | -0.30 | 0.23 | 0.15 | -0.15 | -0.14 | 1.00 | -0.13 | 0.02 |
| $\tau_C$ | 0.05 | 0.02 | 0.28 | -0.18 | 0.14 | -0.03 | -0.11 | -0.17 | 0.06 | -0.24 | 0.16 | 0.21 | -0.00 | -0.10 | -0.00 | -0.01 | -0.06 | -0.13 | -0.13 | 1.00 | 0.11 |
| $\tau_R$ | -0.03 | 0.18 | 0.15 | -0.11 | 0.03 | 0.10 | 0.06 | 0.23 | -0.09 | -0.01 | -0.15 | -0.06 | 0.26 | 0.01 | 0.08 | 0.04 | 0.19 | -0.21 | 0.02 | 0.11 | 1.00 |

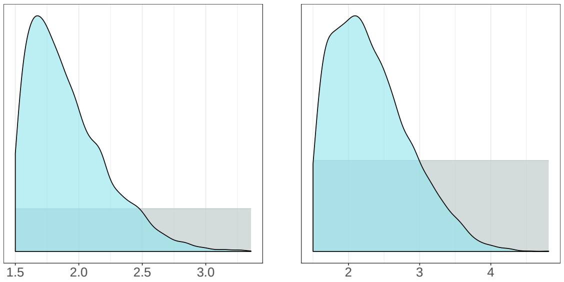


(a) $\tau_C$ : Colon (b) $\tau_R$ : Rectum

Figure 4: Posterior and prior distribution of mean sojoun time parameters.

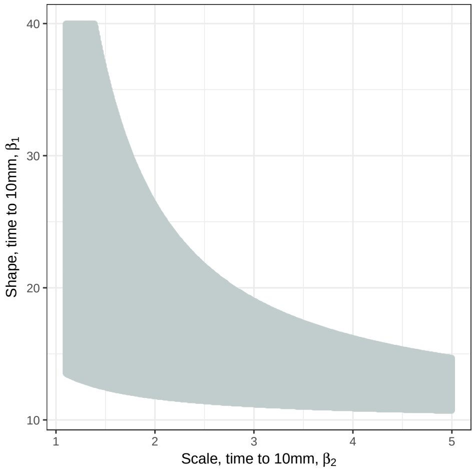


Figure 5: The shaded region shows areas where the restriction on growth parameters is satisfied.

### 1.3 Constraints on Growth Parameters

We restricted growth parameters so that the probability of an adenoma reaching 10mm within 10 years would ranged from 0.0001 to 0.25. This translates to requiring $10(-\ln(0.25))^{1/\beta_1} \leq \beta_2 \leq 10(-\ln(0.0001))^{1/\beta_1}$. Figure 5 shows the effect of this restriction.

### 1.4 Bivariate Contour Plots

In this section we show bivariate posterior distributions for select model parameters demonstrating the correlation of parameters both within and between natural history components.

Within the adenoma risk component (Figure 6), we find correlation between the overall log-risk, $A$, the change in log-risk from ages 20 to 50, modeled by $\alpha_{20}$ and the between-agent standard deviation of adenoma risk ($\sigma_\alpha$). We also find correlation between $\alpha_{20}$ and $\sigma_\alpha$, and between $\alpha_{20}$ and $\alpha_{50}$ In particular, when baseline risk is lower, risk increases more rapidly from 20 to 50 years to accurately predict observed adenoma prevalence, which largely is based on prevalence after age 50 when guidelines recommend initiation of CRC screening (correlation is $-.61$).

Within the adenoma growth component, we find negative correlation between the shape and

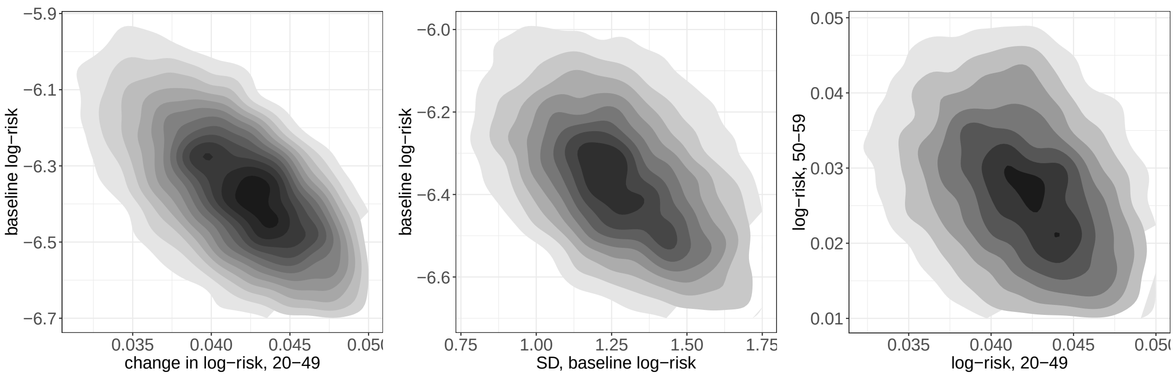


(a) $A$ and $\alpha_{20}$ (b) $A$ and $\alpha_{20}$ (c) $\alpha_{20}$ and $\alpha_{50}$

Figure 6: Bivariate relationships among adenoma risk parameters.

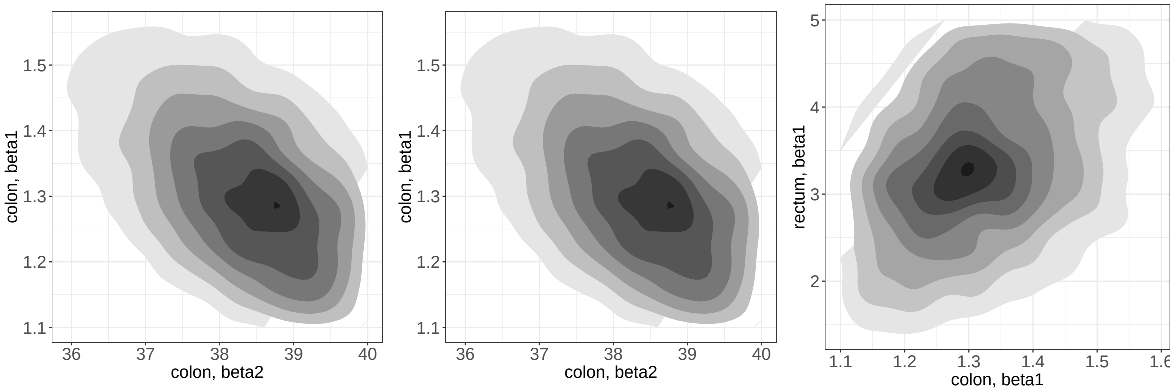


(a) $\beta_{2C}$ and $\beta_{1C}$ (b) $\beta_{2R}$ and $\beta_{1R}$ (c) $\beta_{1R}$ and $\beta_{1C}$

Figure 7: Bivariate relationships among adenoma growth parameters.

scale parameters for adenomas located in the colon (Figure 7; smaller $\beta_2$ reflects faster growth). We also find positive correlation between shape parameters for growth in the colon $\beta_1$ and rectum $\beta_2$ )

The CRC-SPIN model includes eight parameters associated with the transition of adenomas. The overall transition parameter $\gamma_0$ was correlated with several of the adenoma risk parameters, and the age interaction parameters ($\gamma_5$, $\gamma_6$, and $\gamma_7$) are also correlated with each other (Figure **??**). The bivariate distributions of $\gamma_5$, $\gamma_6$, and $\gamma_7$ indicate a relatively flat likelihood, suggesting that these parameter might be dropped from the model (set to zero).

While there was little correlation between $\tau_C$ and $\tau_R$ ($-0.11$), both tended to be near 1.5, the minimum of the prior range (Figure **??**).

There were also relationships among parameters describing different natural history components. For example, correlation between the overall adenoma risk parameter ($A$) and the overall adenoma transition parameter $\gamma_0$ (correlation -0.39, Figure **??**) indicate that when there are more adenomas the overall risk of transition to CRC is lower. In addition, greater variability in adenoma risk across agents corresponds to higher overall transition probabilities. However, for female agents,

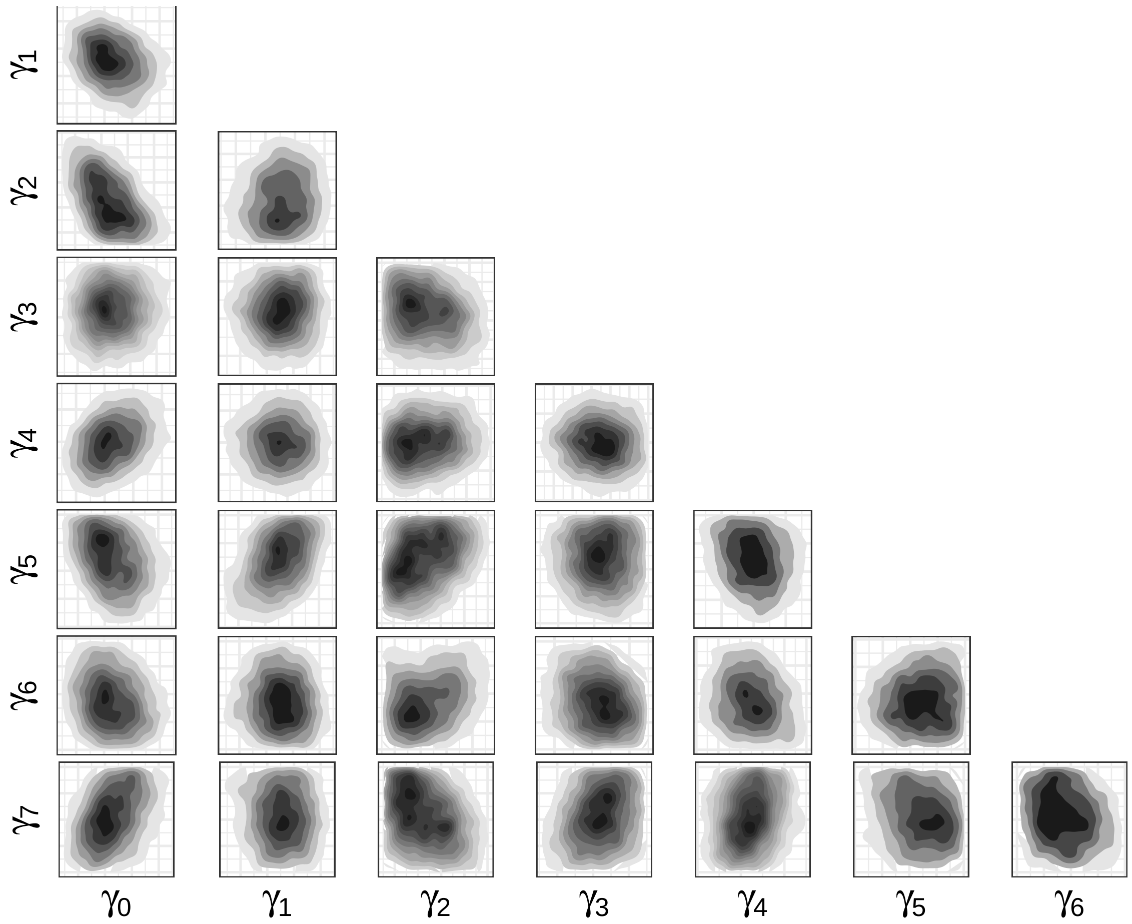


Figure 8: Joint posterior distribution of transition probability parameters.

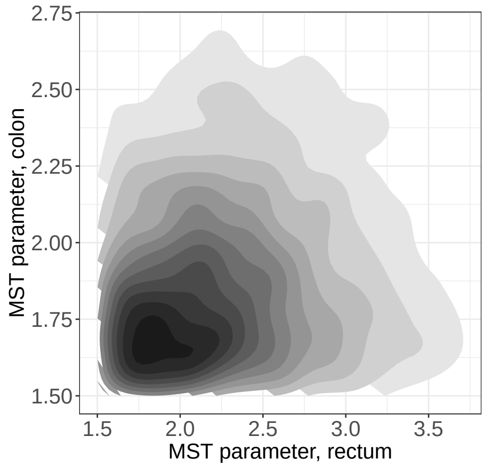


Figure 9: $\tau_R$ and $\tau_C$

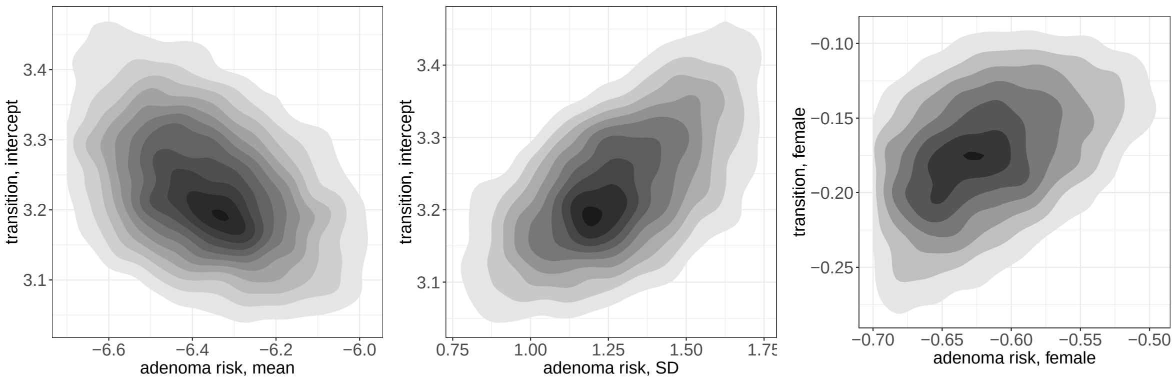


(a) $A$ and $\gamma_0$ (b) $\sigma_\alpha$ and $\gamma_0$ (c) $\alpha_1$ and $\gamma_1$

Figure 10: Bivariate relationships between adenoma risk and transition parameters.

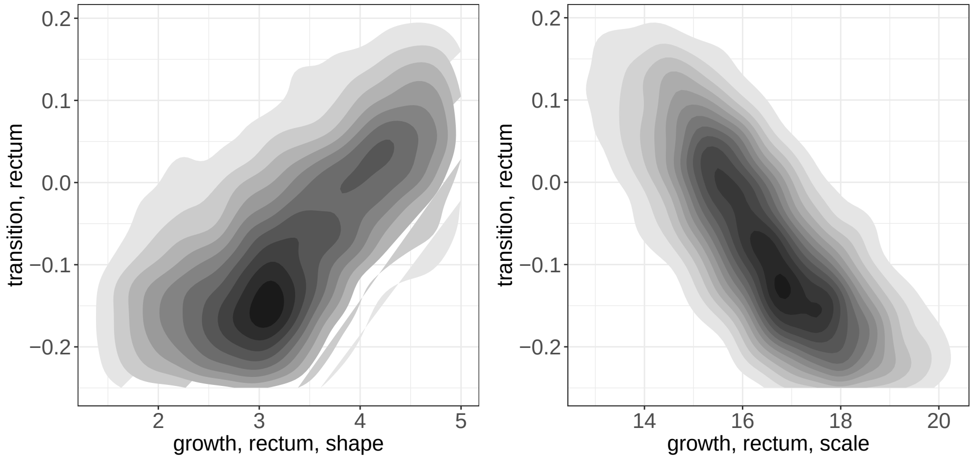


(a) $\beta_{1R}$ and $\gamma_2$ (b) $\beta_{2R}$ and $\gamma_2$

Figure 11: Bivariate relationships between growth and transition parameters for adenoams in the rectum.

increasing adenoma risk corresponds to decreased probabilty of transition (corr($alpha_1$,$\gamma_1$)=0.42). Strong correlation between growth parameters for adenomas in the rectum and the probability of transition to cancer for adenomas in the rectum (Figure **??**) suggests collinearity between these components of the model and the need for more information to tease apart the process of growth and transition probabilties for adenomas in the rectum, such as information about adenoma size by location.

## 1.5 Functions of Model Parameters

Here we provide posterior means and 95% credible intervals for functions of parameters that provide additional information about the model-predicted natural history of CRC. Table 3 provides posterior estimates for the expected time to reach 10 mm for adenomas in the colon and the rec-

tum, as well as the probability that an adenoma in each location reaches 10 mm within 5 years, 10 years, and 20 years. Adenomas in the rectum are faster growing than in the colon, and while the probability that an adenoma reaches 10 mm within 5 years and 10 years is very low for both locations, the probability associated with 20 years is fairly high for rectal cancer.

Table 3: Posterior means and 95% credible intervals for the expected time to reach 10 mm and the probability that an adenoma reaches 10 mm within 5, 10, and 20 years.

| function | location | lower | mean | upper |
|---|---|---|---|---|
| $E(t_{10mm})$ | colon | 89.8 | 160.7 | 332.7 |
| $E(t_{10mm})$ | rectum | 16.3 | 22.9 | 38.3 |
| $Pr(t_{10mm} < 5)$ | colon | 0.0000 | 0.0000 | 0.0000 |
| $Pr(t_{10mm} < 10)$ | colon | 0.0003 | 0.0035 | 0.0099 |
| $Pr(t_{10mm} < 20)$ | colon | 0.07 | 0.10 | 0.12 |
| $Pr(t_{10mm} < 5)$ | rectum | 0.0000 | 0.0001 | 0.0003 |
| $Pr(t_{10mm} < 10)$ | rectum | 0.0002 | 0.0177 | 0.0956 |
| $Pr(t_{10mm} < 20)$ | rectum | 0.40 | 0.60 | 0.83 |

Table 4 provides the mean and 95% credible intervals for the probability that an adenoma in the colon or rectum transitions to preclinical cancer within 5, 10, and 15 mm, for adenomas initiated at age 40 for men and women.

Table 5 provides inference for mean sojourn time and the probability that sojourn time is less than 1 year, less than 2 years, and greater than 4 years, for cancer in the colon and rectum.

Table 4: The probability that an adenoma in the colon and rectum transitions to preclinical cancer within 5, 10, and 20 mm, for adenomas initiated at age 40 for men and women.

| size | sex | location | lower | mean | upper |
|---|---|---|---|---|---|
| 5mm | female | colon | 0.0001 | 0.0005 | 0.0014 |
| 10mm | female | colon | 0.01 | 0.03 | 0.05 |
| 20mm | female | colon | 0.18 | 0.30 | 0.41 |
| 5mm | female | rectum | 0.0001 | 0.0004 | 0.0016 |
| 10mm | female | rectum | 0.01 | 0.02 | 0.06 |
| 20mm | female | rectum | 0.14 | 0.26 | 0.42 |
| 5mm | male | colon | 0.0000 | 0.0001 | 0.0003 |
| 10mm | male | colon | 0.00 | 0.01 | 0.02 |
| 20mm | male | colon | 0.10 | 0.19 | 0.28 |
| 5mm | male | rectum | 0.0000 | 0.0002 | 0.0008 |
| 10mm | male | rectum | 0.01 | 0.02 | 0.04 |
| 20mm | male | rectum | 0.12 | 0.22 | 0.34 |

Table 5: Mean sojourn time and the probability that sojourn time is less than 1 year, less than 2 years, and greater than 4 years, for cancer in the colon and rectum.

| function | location | lower | mean | upper |
|---|---|---|---|---|
| mean | colon | 1.39 | 1.75 | 2.40 |
| mean | rectum | 1.42 | 2.12 | 3.26 |
| prob $<$ 1 yr. | colon | 0.01 | 0.05 | 0.12 |
| prob $<$ 2 yr. | colon | 0.23 | 0.72 | 0.98 |
| prob $>$ 4 yr. | colon | 0.0000 | 0.0002 | 0.0004 |
| prob $<$ 1 yr. | rectum | 0.00 | 0.03 | 0.11 |
| prob $<$ 2 yr. | rectum | 0.05 | 0.48 | 0.97 |
| prob $>$ 4 yr. | rectum | 0.0000 | 0.0136 | 0.1624 |

## References


Church, J. M. (2004), "Clinical Significance of Small Colorectal Polyps," *Dis Colon Rectum*, 47, 481–485.

Corley, D. A., Jensen, C. D., Marks, A. R., Zhao, W. K., De Boer, J., Levin, T. R., Doubeni, C., Fireman, B. H., and P, Q. C. (2013), "Variation of Adenoma Prevalence by Age, Sex, Race adn colon Location in a Large Population: Implications for Screening and Quality Programs," *Clinical Gastroenterology and Hepatology*, 11, 172–180.

Lieberman, D. A., Weiss, D. G., Bond, J. H., Ahnen, D. J., Garewal, H., and Chejfec, G. (2000), "Use of Colonoscopy to Screen Asymptomatic Adults for Colorectal Cancer," *NEJM*, 343, 162–168.

Lieberman, D., Moravec, M., Holub, J., Michaels, L., and Eisen, G. (2008), "Polyp Size and Advanced Histology in Patients Undergoing Colonoscopy Screening: Implications for CT Colonography," *Gastroenterology*, 135, 1100–1105.

Pickhardt, P. J., Choi, R., Hwang, I., Butler, J. A., Puckett, M. L., Hildebrandt, H. A., Wong, R. K., Nugent, P. A., Mysliwiec, P. A., and Schindler, W. R. (2003), "Computed Tomographic Virtual Colonocopy to Screen for Colorectal Neoplasia in Asymptomatic Adults," *NEJM*, 349, 2191–2200.
